# Supplementary material for: Analysing Meso and Macro conversation structures in an online suicide support forum
Source: arXiv:2007.10159 source file (2020-07-20)
Supplement: Supplementary file 3 [file Supplementary.pdf]

# Analysing network structures of conversations in an online suicide support forum

Sagar Joglekar<sup>1</sup>, Sumithra Velupillai<sup>1,2</sup>, Rina Dutta<sup>2</sup>, and  
Nishanth Sastry<sup>1</sup>

<sup>1</sup>King's College, Department of Informatics, London, UK

<sup>2</sup>King's College London, IoPPN, London, SE5 8AF, UK

## **Supplementary material**

We performed motif census for all the 36 Anchored triadic motifs across all BL and FP datasets. Figure 0 exhibits the trends in anchored motif census, for the insignificantly expressed or equally prevalent motifs.

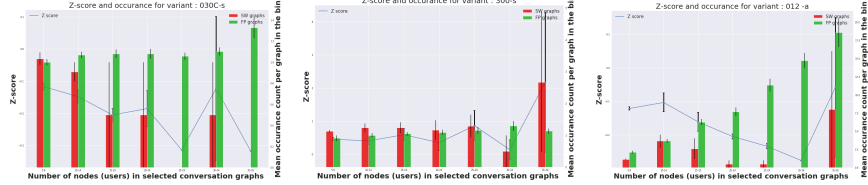

(1.a)

(1.b)

(1.c)

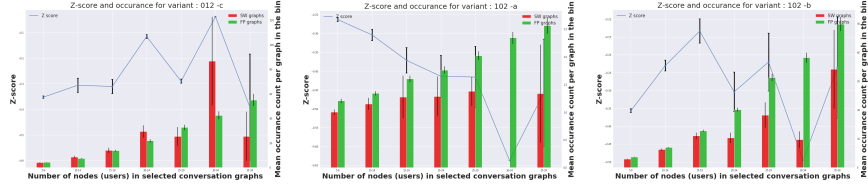

(2.a)

(2.b)

(2.c)

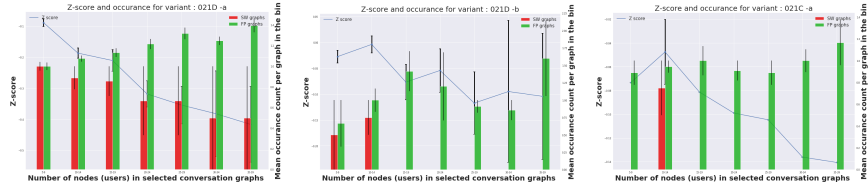

(3.a)

(3.b)

(3.c)

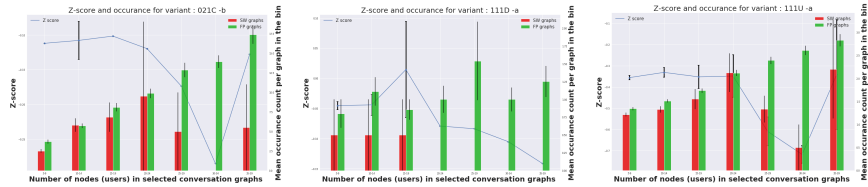

(4.a)

(4.b)

(4.c)

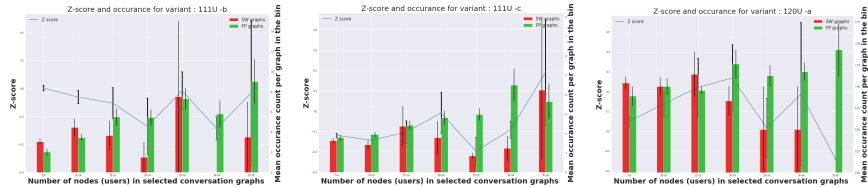

(5.a)

(5.b)

(5.c)

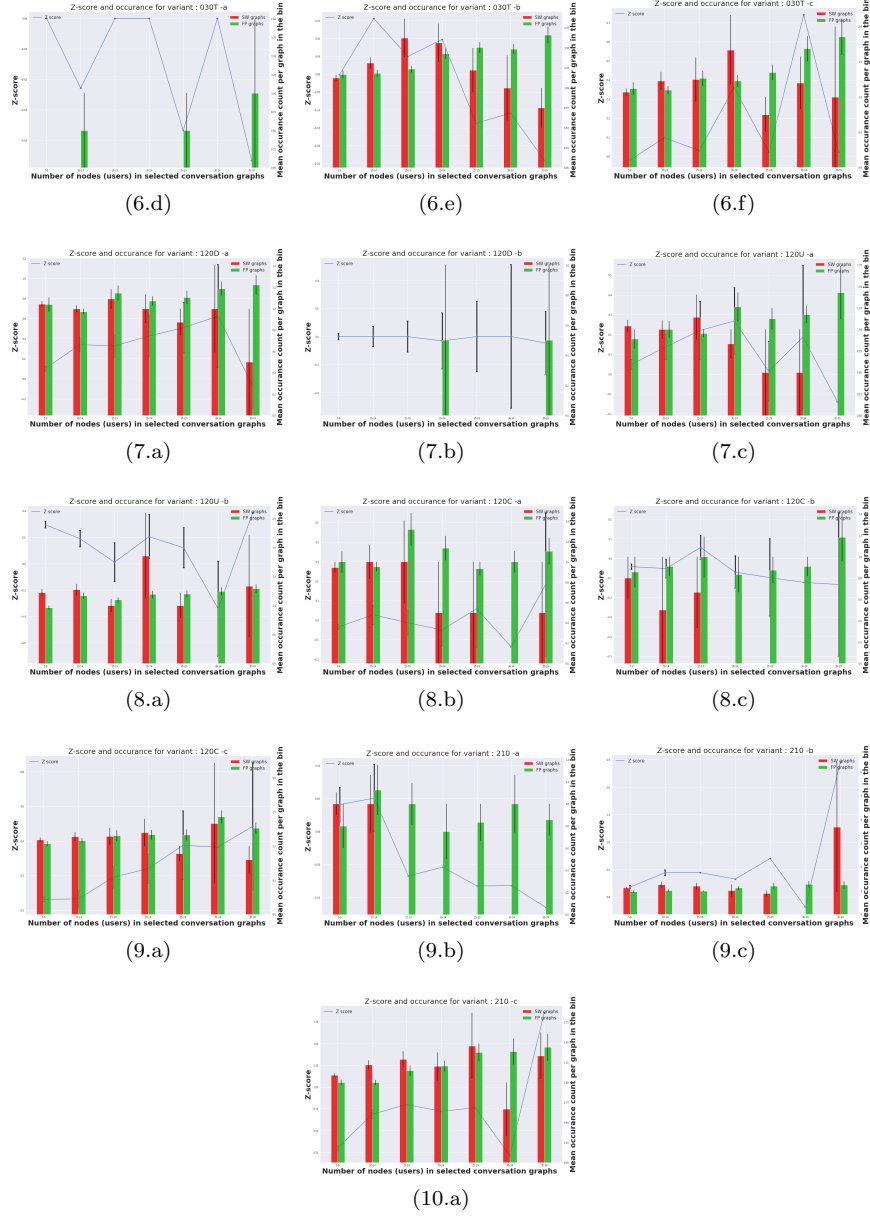

Figure 0: This figure lists all the insignificant Anchored motifs, either by the virtue of rare occurrence ( $<10$  mean motifs per bin) or by account of low Z-score ( $|Z| < 1$ ).
